# Supplementary material for: EvPlug: Learn a Plug-and-Play Module for Event and Image Fusion
Source: arXiv:2312.16933 source file (2023-12-28)
Supplement: Supplementary file 1 [file neurips_2023_supp.tex]

% \documentclass{article}


% % if you need to pass options to natbib, use, e.g.:
% %     \PassOptionsToPackage{numbers, compress}{natbib}
% % before loading neurips_2023


% % ready for submission
% % \usepackage{neurips_2023}


% % to compile a preprint version, e.g., for submission to arXiv, add add the
% % [preprint] option:
% %     \usepackage[preprint]{neurips_2023}


% % to compile a camera-ready version, add the [final] option, e.g.:
% %     \usepackage[final]{neurips_2023}


% % to avoid loading the natbib package, add option nonatbib:
% \usepackage[nonatbib]{neurips_2023}


% \usepackage[utf8]{inputenc} % allow utf-8 input
% \usepackage[T1]{fontenc}    % use 8-bit T1 fonts
% \usepackage{hyperref}       % hyperlinks
% \usepackage{url}            % simple URL typesetting
% \usepackage{booktabs}       % professional-quality tables
% \usepackage{amsfonts}       % blackboard math symbols
% \usepackage{nicefrac}       % compact symbols for 1/2, etc.
% \usepackage{microtype}      % microtypography
% \usepackage{xcolor}         % colors
% \usepackage{graphicx}
% \usepackage{animate}
% \usepackage{float}
% \usepackage{amsmath}
% \usepackage{amssymb}
% \usepackage[ruled,vlined]{algorithm2e}
% \usepackage{multirow}
% \usepackage{colortbl}
% \usepackage{array}
% \usepackage{makecell}
% \usepackage{bbding}
% \usepackage{enumitem}
% \usepackage{caption}
% \usepackage{tabularx}
% \usepackage{subfig}

% \def\loss{{\mathcal{L}}}
% \newcommand{\jianping}[1]{\textcolor{blue}{{[Jianping: #1]}}}


% \newcommand{\Tref}[1]{Tab.~\ref{#1}}
% \newcommand{\Eref}[1]{Eq.~(\ref{#1})}
% \newcommand{\Fref}[1]{Fig.~\ref{#1}}
% \newcommand{\Sref}[1]{Sec.~\ref{#1}}
% \newcommand{\Aref}[1]{Alg.~\ref{#1}}

% \def\onedot{.}
% \def\eg{\emph{e.g}\onedot} \def\Eg{\emph{E.g}\onedot}
% \def\ie{\emph{i.e}\onedot} \def\Ie{\emph{I.e}\onedot}
% \def\cf{\emph{c.f}\onedot} \def\Cf{\emph{C.f}\onedot}
% \def\etc{\emph{etc}\onedot} \def\vs{\emph{vs}\onedot}
% \def\wrt{w.r.t\onedot} \def\dof{d.o.f\onedot}
% \def\etal{\emph{et al}\onedot}

% \newcommand{\methodnamenocolor}{EvPlug}

% \newcommand{\methodname}[1]{\textbf{EvPlug}}
% % \def\methodnamenocolor{\textbf{{EvPlug}}}
% \def\degradation{XXX}
% \def\sequential{XXXXXX}

% \title{Supplemental Materials:\\\methodnamenocolor{}: Learn a Plug-and-Play Module for Event and Image Fusion}


% % The \author macro works with any number of authors. There are two commands
% % used to separate the names and addresses of multiple authors: \And and \AND.
% %
% % Using \And between authors leaves it to LaTeX to determine where to break the
% % lines. Using \AND forces a line break at that point. So, if LaTeX puts 3 of 4
% % authors names on the first line, and the last on the second line, try using
% % \AND instead of \And before the third author name.


% \author{%
%  Jianping Jiang \\
%   Department of Computer Science\\
%   xx University\\
%   \texttt{hippo@cs.cranberry-lemon.edu} \\
%   % examples of more authors
%   % \And
%   % Coauthor \\
%   % Affiliation \\
%   % Address \\
%   % \texttt{email} \\
%   % \AND
%   % Coauthor \\
%   % Affiliation \\
%   % Address \\
%   % \texttt{email} \\
%   % \And
%   % Coauthor \\
%   % Affiliation \\
%   % Address \\
%   % \texttt{email} \\
%   % \And
%   % Coauthor \\
%   % Affiliation \\
%   % Address \\
%   % \texttt{email} \\
% }


% \setcounter{figure}{9}
% \setcounter{table}{3}
% \setcounter{section}{5}

% \begin{document}


% \maketitle




% \section{Multi-modal Fusion Module}

% Our multi-modal fusion module $f_{\text{E-Former}}$, as shown in \Fref{fig: e-former}, uses the structure of the transformer decoder layer~\cite{vaswani17transformer}. Since the transformer can model long-term sequential information~\cite{vaswani17transformer} and non-local spatial information~\cite{carion20detr, doso21vit}, we use a unified $f_{\text{E-Former}}$ to ensure event-image quality and temporal consistency during the fusion process of events and images. Borrowing the concept from Perceiver~\cite{perceiver21}, $f_{\text{E-Former}}$ can flexibly set the number of self-attention layers in each transformer block, and also the number of transformer blocks. In our experiment, we use the same parameters of $f_{\text{E-Former}}$ as DETR~\cite{carion20detr} (feed forward dimension: 1024, number of head: 4, position encoding type: sine, dropout rate: 0.1), and keep them consistent in all three downstream tasks.

% \begin{figure}[h]
%   \centering
%    \includegraphics[width=\textwidth]{data/supp/e-former.pdf}
%   \caption{Illustration to the details of $f_{\text{E-Former}}$, where K, Q, V represent the key, query, and value of the multi-head self-attention (MHSA). N is the number of transformer decoder layers.
%   }
%   \label{fig: e-former}
%   \vspace{-0.cm}
% \end{figure}  




% \section{Additional Experiment Results}

% We show additional qualitative results to complement the results in the main paper.

% As shown in \Fref{fig: add quality od}, \methodname{}, compared to RGB-based methods, can precisely detect distant small objects, thanks to the rich motion information integrated by $f_{\text{E-Former}}$ from the event stream. In contrast to event-based methods and domain adaptation methods~\cite{gehrig20v2e, hu20nga, messikommer22evtransfer}, \methodname{} leverages the effective texture and color information from images, demonstrating a strong perception capability for nearby objects.


% \begin{figure}[h]
%   \centering
%     % \vspace{-0.1cm}
%   \includegraphics[width=\textwidth]{data/supp/od_supp.pdf}
%   \begin{flushleft}
%     \scriptsize  \hspace{0.6cm}RGB(GT) \hspace{0.55cm} Event-based~\cite{carion20detr} \hspace{0.7cm} NGA~\cite{hu20nga} \hspace{0.85cm} E2VID~\cite{rebecq21e2vid} \hspace{0.6cm} EvTransfer~\cite{messikommer22evtransfer}  \hspace{0.4cm} RGB-based~\cite{carion20detr} \hspace{0.7cm} \methodname{}
%   \end{flushleft}
%   \caption{Additional qualitative results on DSEC-MOD~\cite{zhou2023rgb}.}
%   \label{fig: add quality od}
% \end{figure}

% In \Fref{fig: add quality ss}, we show that \methodname{} can effectively recognize the edges of buildings and trees due to the texture information in RGB images, while domain adaptation methods~\cite{gehrig20v2e, hu20nga, messikommer22evtransfer} cannot deal with these categories with only event streams.


% \begin{figure}[h]
%   \centering
%   \includegraphics[width=\textwidth]{data/supp/ss_supp.pdf}
%   \begin{flushleft}
% \scriptsize  \hspace{0.5cm}RGB \hspace{0.8cm} Events \hspace{0.9cm} GT \hspace{0.65cm}Ev-SegNet~\cite{alonso19evsegnet}\hspace{0.45cm}NGA~\cite{hu20nga} \hspace{0.45cm} E2VID~\cite{rebecq21e2vid} \hspace{0.2cm} EvTransfer~\cite{messikommer22evtransfer}  \hspace{0.25cm} DETR~\cite{carion20detr} \hspace{0.45cm} \methodname{}
%   \end{flushleft}
%   \caption{Additional qualitative results on DSEC-Semantic~\cite{sun22ess}.}
%   \label{fig: add quality ss}
%   % \vspace{-0.2cm}
% \end{figure}

% As shown in \Fref{fig: add quality hpe}, when the event-based method~\cite{victor21eventhands} and domain adaptation methods~\cite{gehrig20v2e, hu20nga, messikommer22evtransfer} cannot estimation precise hand meshes when the edges of fingers are occluded by each other or obstructed by the illumination changes. \methodname{} can integrate both texture information from RGB images and motion information from event streams for robust hand pose estimation.


% \begin{figure}[h]
%   % \vspace{-0.5cm}
%   \centering
%   \includegraphics[width=\textwidth]{data/supp/hpe_supp.pdf}
%       \begin{flushleft}
%     \scriptsize  \hspace{.7cm}RGB \hspace{0.95cm} Events \hspace{0.4cm} EventHands~\cite{victor21eventhands} \hspace{0.35cm}  NGA~\cite{hu20nga} \hspace{0.55cm} E2VID~\cite{rebecq21e2vid} \hspace{0.5cm} EvTransfer~\cite{messikommer22evtransfer} \hspace{0.25cm} FastMETRO~\cite{cho22fastmetro}  \hspace{0.4cm} \methodname{}
%   \end{flushleft}
%    \caption{Addtional qualitative results on EvRealHands~\cite{jiang23evhandpose}.}
%   \label{fig: add quality hpe}
%   % \vspace{-0.2cm}
% \end{figure}











% {\small
% \bibliographystyle{ieee_fullname}
% \bibliography{egbib}
% }



% \end{document}
